# Supplementary material for: Learning Representations by Humans, for Humans
Source: arXiv:1905.12686 source file (2021-09-15)
Supplement: Supplementary file 1 [file tmp_supp.tex]

\clearpage
\onecolumn
%\makeappendixtitle
\appendix

\begin{appendices}

\section{Optimization Algorithm} \label{sec:algo}

\section{General Optimization Issues} \label{sec:opt}

\subsection{Initialization}

\subsection{Convergence}


\subsection{Regularization/Early Stopping}

\subsection{Human Input}

\section{Experimental Details}



\subsection{Decision-compatible 2D projections} \label{sec:exp1}


\subsection{Decision-compatible algorithmic avatars} \label{sec:exp3}

\subsubsection{Data Preprocessing.}

\subsubsection{Learning architecture and pipeline.} \label{sec:exp3details}

\subsubsection{Self-reported user type.}

\subsubsection{Diversity in avatar representation.} \label{sec:avatarreps}

\subsubsection{Further Details on Information Learned by $z$.}


\subsection{Incorporating Side Information} \label{sec:exp2}


\subsubsection{Data Generation.} \label{sec:side_info_data_gen}

\subsubsection{Learning Architecture.}


\subsubsection{Baselines.} 

\section{Select Turker quotes}

\end{appendices}
